# Supplementary material for: K12Vista: Exploring the Boundaries of MLLMs in K-12 Education
Source: arXiv:2506.01676 source file (2026-11-25)
Supplement: Supplementary file 1 [file appendix_ablation_more_model_as_evaluation.tex]

\begin{wraptable}[15]{r}{0.49\textwidth} % [13] 表示表格所占文本行数，r 表示右对齐
    \centering
    \caption{The Statistic of \ours} 
    \begin{tabular}{lccccccccccc} 
        \toprule 
        Statistic & \#Number \\
        \midrule 
        Question Number & 33,660 \\
        Total Subjects & 5 \\
        Total Knowledge Points & 17721  \\
        Total Question Types & 3 \\
        \midrule 
        Average Problem Tokens & 150.44 \\
        Average Reference Solution Tokens & 247.48 \\
        Average Reference Solution Steps & 5.15 \\
        Average Number of Answers & 3.24 \\
        Average Answer Tokens & 24.88 \\
        \bottomrule 
    \end{tabular}
    \label{tab:Statisitc table} 
\end{wraptable}
