# Supplementary material for: K12Vista: Exploring the Boundaries of MLLMs in K-12 Education
Source: arXiv:2506.01676 source file (2026-11-25)
Supplement: Supplementary file 2 [file appendix_error_list.tex]

\begin{table}[!t]
\caption{Performance of MLLMs across Primary, Middle, and High School Grades under Direct Inference and CoT Reasoning Step-by-Step Evaluation. Overall performance represents the average accuracy across all questions.}
\centering
\begin{tabular}{p{4cm} p{8cm}}
    \hline
    \textbf{Error Types} & \textbf{Definitions} \\
    \hline
    Image Cognition Error & Misidentification in understanding charts, graphs, objects, or spatial relationships .\\
    \hline
    Question Misunderstanding & Errors due to misunderstanding question requirements, conditions, or key information .\\
    \hline
    Lack of Relevant Knowledge & Inability to understand or integrate subject knowledge .\\
    \hline
    Knowledge Application Error & Errors from flawed mastery or misinterpretation of concepts, principles, formulas, or methods .\\
    \hline
    Logical Reasoning Error & Systematic errors in reasoning .\\
    \hline
    Hallucination Error & Factual errors, logical inconsistencies, or unwarranted inferences .\\
    \hline
    Calculation Error & Specific mistakes in mathematical operations or algebraic manipulations .\\
    \hline
    Incomplete Answer Error & Failing to provide a final answer or omitting parts of the answer.\\
    \hline
\end{tabular}
\label{tab:appendix_error_list}
\end{table}
